# Supplementary material for: KG-HTC: Integrating Knowledge Graphs into LLMs for Effective Zero-shot Hierarchical Text Classification
Source: arXiv:2505.05583 source file (2025-05-08)
Supplement: Supplementary file 1 [file appendix.tex]

Finally, real-world datasets predominantly manifest long-tail distribution problems, where such imbalanced data characteristics substantially compromise the generalization of classification models.
As Figure~\ref{fig:long_tail} shows, statistical analysis reveals that the top 15\% most frequent categories account for 80\% of total instances in the third level of the Amazon Product Review dataset. In contrast, the bottom 50\% sparse categories collectively represent merely 6\% of the data volume.

\begin{figure*}[t]
    \centering
    \refstepcounter{picturecounter}
    \label{fig:long_tail}
    \includegraphics[width=1\linewidth]{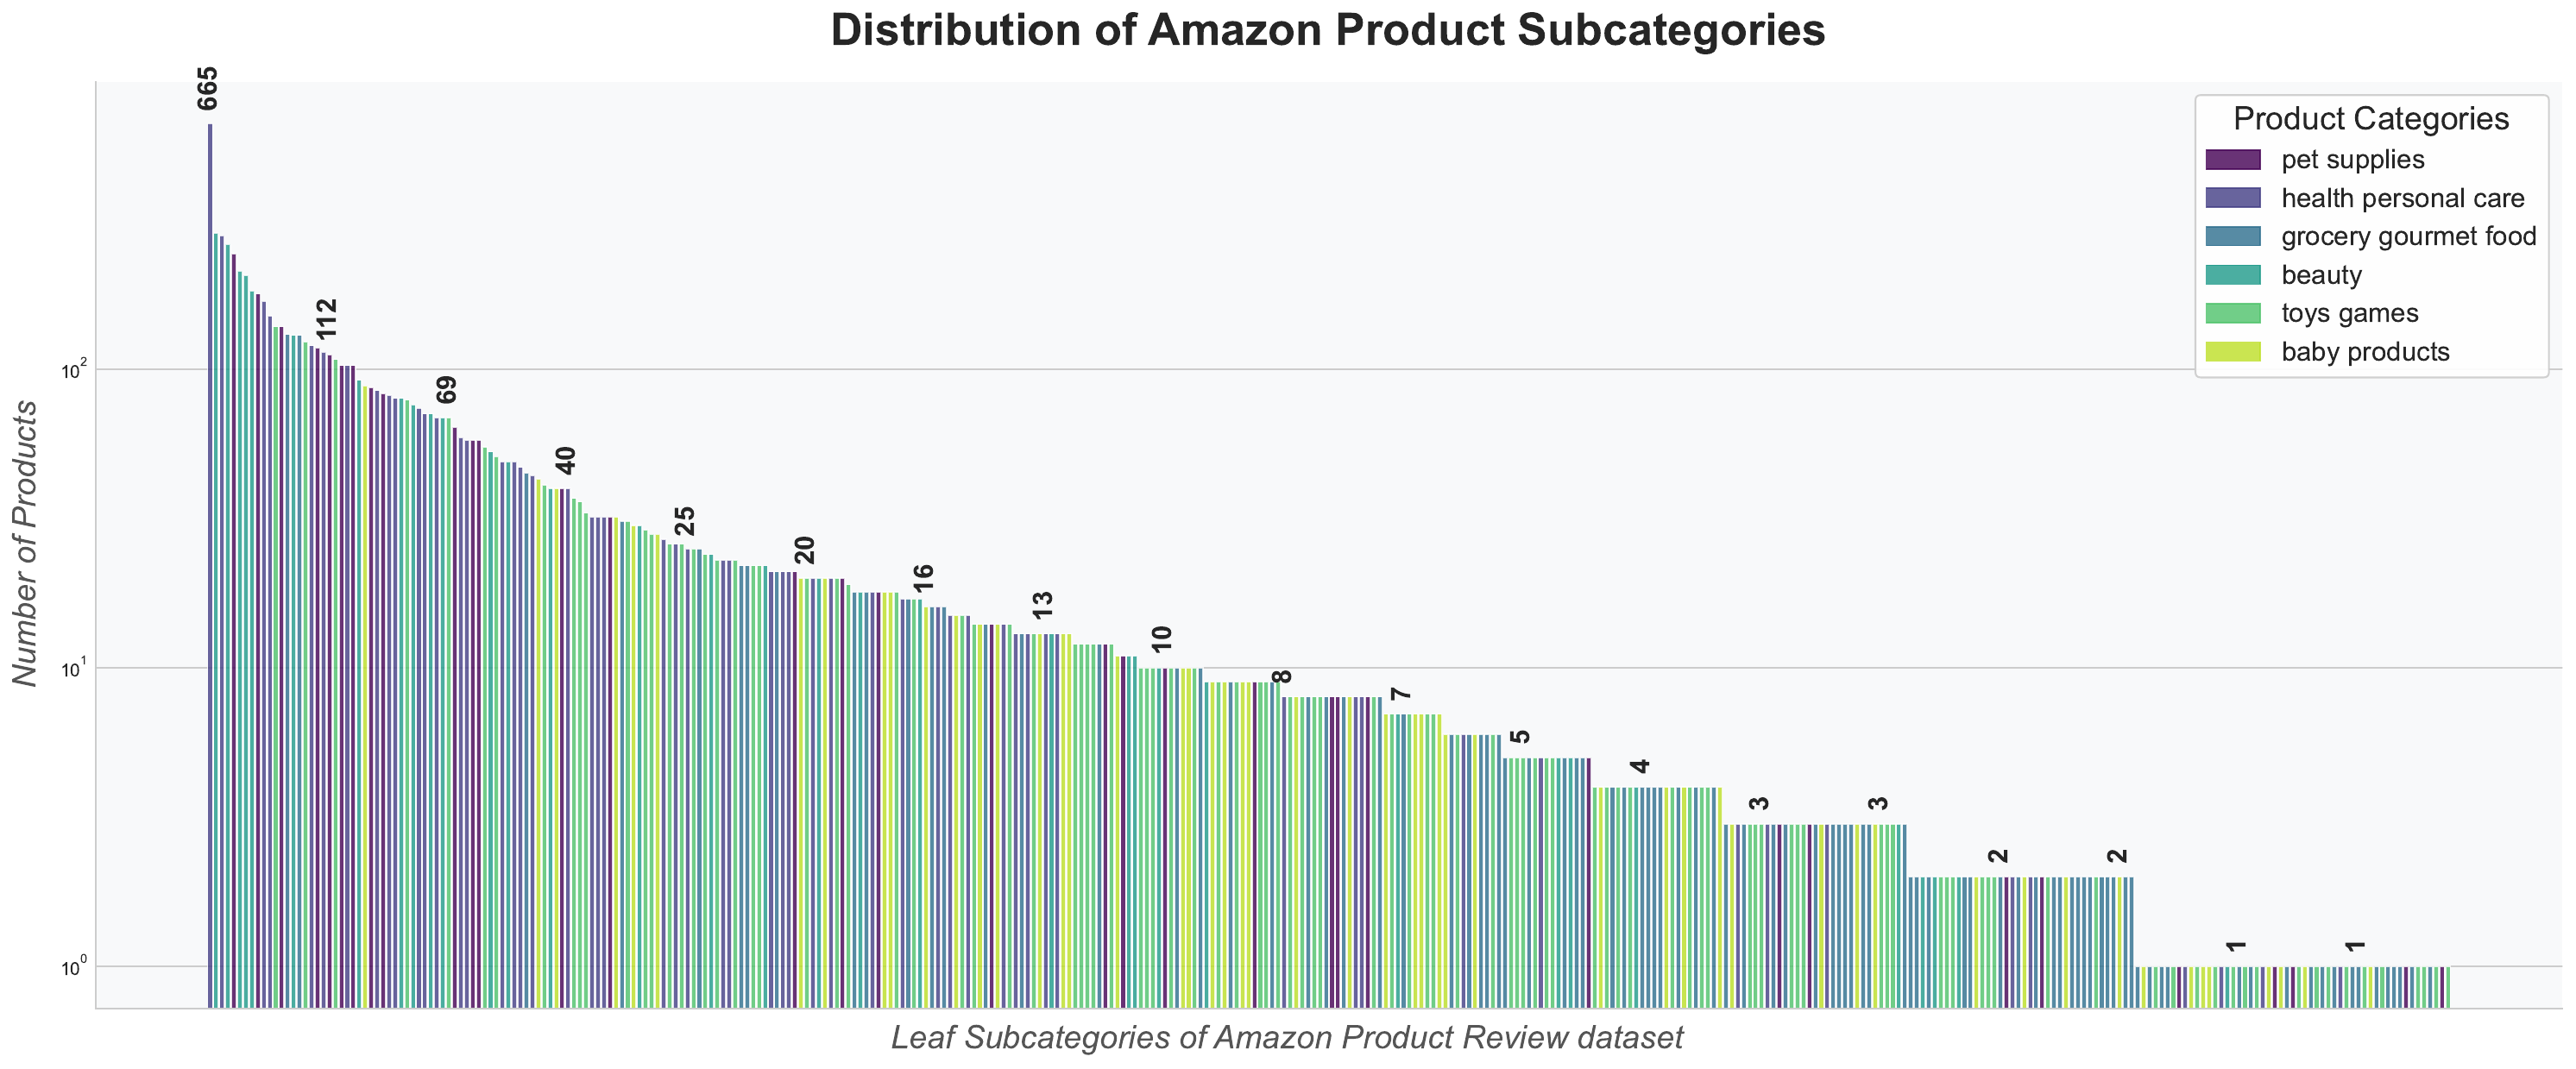}
    \caption{The long-tail distribution problem from the Amazon Product Review dataset. Statistical analysis reveals that the top 15\% most frequent categories account for 80\% of total instances in the third level.}
    \vspace{20pt}
\end{figure*}
